# Supplementary material for: Data-driven shape inference in three-dimensional steady state supersonic flows using ODIL and JAX-Fluids
Source: arXiv:2408.10094 source file (2025-06-18)
Supplement: Supplementary file 2 [file flowfield_rho.tex]

\begin{tikzpicture}
    % \pgfmathdeclarefunction{lg10}{1}{%
    %     \pgfmathparse{ln(#1)/ln(10)}%
    % }
    
    % Spectral_r colormap from matplotlib
    \pgfplotsset{
        colormap={spectralr}{rgb255=(94,79,162) rgb255=(68,112,177) rgb255=(59,146,184) rgb255=(89,180,170)
            rgb255=(126,203,164) rgb255=(166,219,164) rgb255=(202,233,157) rgb255=(232,246,156) 
            rgb255=(247,252,179) rgb255=(254,245,175) rgb255=(254,227,145) rgb255=(253,200,119) 
            rgb255=(252,170,95) rgb255=(247,131,77) rgb255=(236,97,69) rgb255=(218,70,76)
            rgb255=(190,36,73) rgb255=(158,1,66)}}
    
    \begin{groupplot}[
        group style={
            group size=4 by 2,
            horizontal sep=0.8cm,
            vertical sep=2.0cm
        }, 
        width=4.2cm, 
        height=4.2cm
        ]
        \nextgroupplot[
            tick align=outside,
            tick pos=left,
            xtick style={draw=none},
            ytick style={draw=none},
            xticklabels = {},
            xtick = {},
            yticklabels = {},
            ytick = {},
            % title=$\rho$,
            title=ODIL,
            enlargelimits=false,
            colormap name=spectralr,
            axis equal image,
            colorbar,
            colorbar horizontal,
            colorbar style={
                at={(0.0,-0.05)},
                anchor=north west,
                xtick style={
                    draw=none,
                },
                xtick={1.0,1.24,1.48},
                xticklabels = {1.00,1.24,1.48},
                height=0.2cm
            },
            point meta min=1.0,
            point meta max=1.48
        ]
        \addplot graphics [xmin=-0.3,xmax=0.3,ymin=-0.3,ymax=0.3] {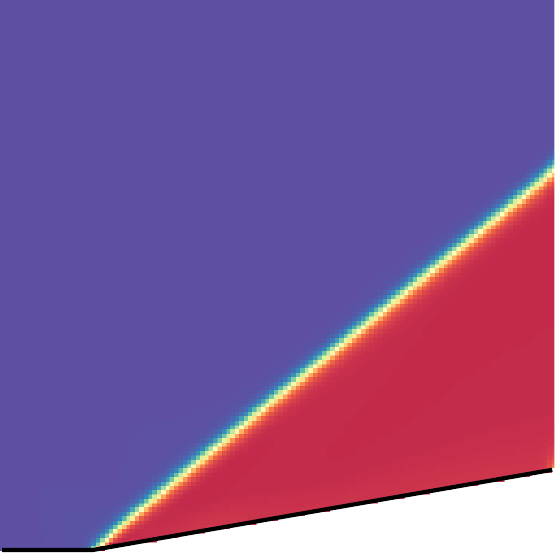};

        \nextgroupplot[
            tick align=outside,
            tick pos=left,
            xtick style={draw=none},
            ytick style={draw=none},
            xticklabels = {},
            xtick = {},
            yticklabels = {},
            ytick = {},
            title=discrete ref.,
            enlargelimits=false,
            colormap name=spectralr,
            axis equal image,
            colorbar,
            colorbar horizontal,
            colorbar style={
                at={(0.0,-0.05)},
                anchor=north west,
                xtick style={
                    draw=none,
                },
                xtick={1.0,1.24,1.48},
                xticklabels = {1.00,1.24,1.48},
                height=0.2cm
            },
            point meta min=1.0,
            point meta max=1.48
        ]
        \addplot graphics [xmin=-0.3,xmax=0.3,ymin=-0.3,ymax=0.3] {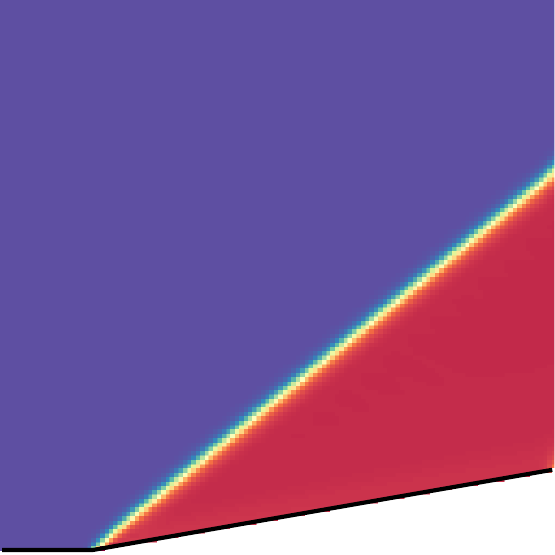};

        \nextgroupplot[
            tick align=outside,
            tick pos=left,
            xtick style={draw=none},
            ytick style={draw=none},
            xticklabels = {},
            xtick = {},
            yticklabels = {},
            ytick = {},
            title=$\log_{10}$(|rel. error|),
            enlargelimits=false,
            colormap name=spectralr,
            colorbar,
            colorbar horizontal,
            colorbar style={
                at={(0.0,-0.05)},
                anchor=north west,
                xtick style={
                    draw=none,
                },
                xtick={-6,-3,0},
                height=0.2cm
            },
            point meta min=-6,
            point meta max=0
        ]
        \addplot graphics [xmin=-0.3,xmax=0.3,ymin=-0.3,ymax=0.3] {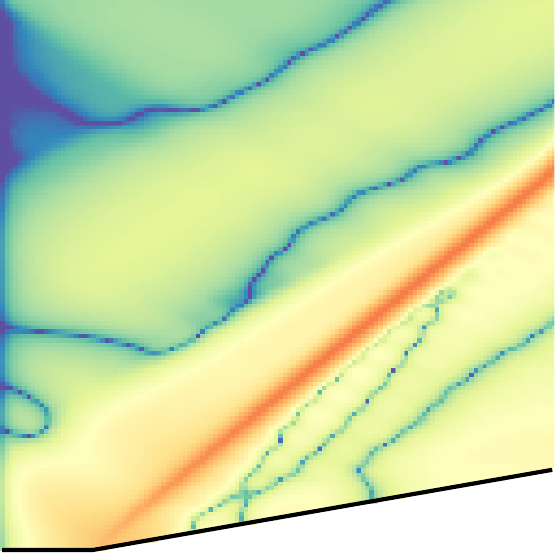};

        \nextgroupplot[
            tick align=outside,
            tick pos=left,
            xshift=1cm,
            ymin=1e-6,
            ymax=1e4,
            log basis x={10},
            log basis y={10},
            ymode=log,
            xtick style={color=black},
            xlabel=step,
            % ylabel=$\mathcal{L}$,
            title=$\omega \mathcal{L}$,
            ]
        \addplot [line width=1.0pt, TUMblue] table[x index = {0}, y index = {1}]
        {figures/appendix/forward_problem/odil/loss_history_100000.txt};
        \addplot [line width=1.0pt, black, dashed] coordinates {(50000,1e-6) (50000,1e4)};
        \nextgroupplot[
            tick align=outside,
            tick pos=left,
            xtick style={draw=none},
            ytick style={draw=none},
            xticklabels = {},
            xtick = {},
            yticklabels = {},
            ytick = {},
            % title=$\rho$,
            title=PINN,
            enlargelimits=false,
            colormap name=spectralr,
            axis equal image,
            colorbar,
            colorbar horizontal,
            colorbar style={
                at={(0.0,-0.05)},
                anchor=north west,
                xtick style={
                    draw=none,
                },
                xtick={1.0,1.23,1.46},
                xticklabels = {1.00,1.23,1.46},
                height=0.2cm
            },
            point meta min=1.0,
            point meta max=1.46
        ]
        \addplot graphics [xmin=-0.3,xmax=0.3,ymin=-0.3,ymax=0.3] {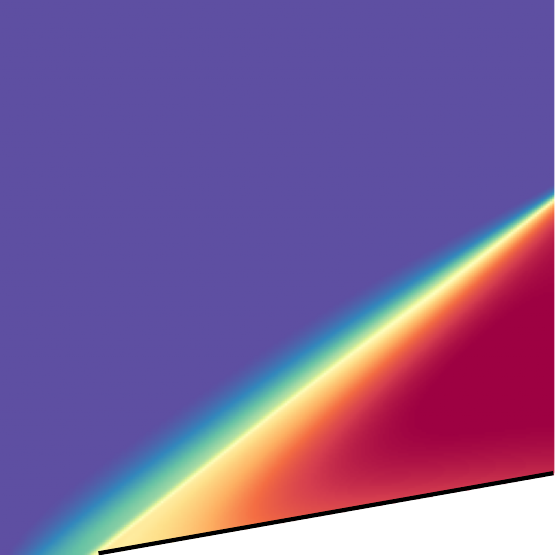};

        \nextgroupplot[
            tick align=outside,
            tick pos=left,
            xtick style={draw=none},
            ytick style={draw=none},
            xticklabels = {},
            xtick = {},
            yticklabels = {},
            ytick = {},
            title=analytical ref.,
            enlargelimits=false,
            colormap name=spectralr,
            axis equal image,
            colorbar,
            colorbar horizontal,
            colorbar style={
                at={(0.0,-0.05)},
                anchor=north west,
                xtick style={
                    draw=none,
                },
                xtick={1.0,1.23,1.46},
                xticklabels = {1.00,1.23,1.46},
                height=0.2cm
            },
            point meta min=1.0,
            point meta max=1.46
        ]
        \addplot graphics [xmin=-0.3,xmax=0.3,ymin=-0.3,ymax=0.3] {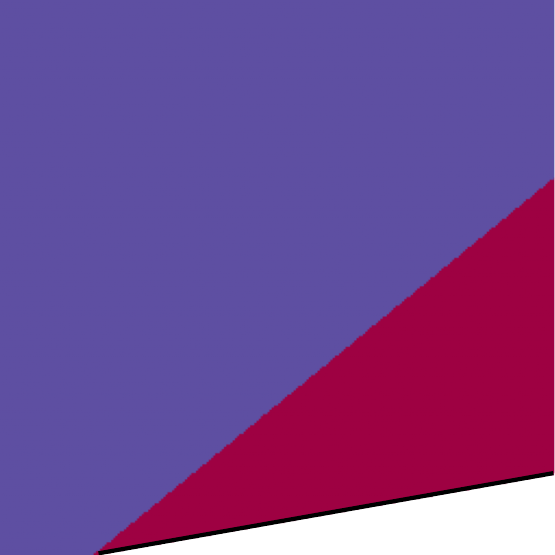};

        \nextgroupplot[
            tick align=outside,
            tick pos=left,
            xtick style={draw=none},
            ytick style={draw=none},
            xticklabels = {},
            xtick = {},
            yticklabels = {},
            ytick = {},
            title=$\log_{10}$(|rel. error|),
            enlargelimits=false,
            colormap name=spectralr,
            colorbar,
            colorbar horizontal,
            colorbar style={
                at={(0.0,-0.05)},
                anchor=north west,
                xtick style={
                    draw=none,
                },
                xtick={-6,-3,0},
                height=0.2cm
            },
            point meta min=-6,
            point meta max=0
        ]
        \addplot graphics [xmin=-0.3,xmax=0.3,ymin=-0.3,ymax=0.3] {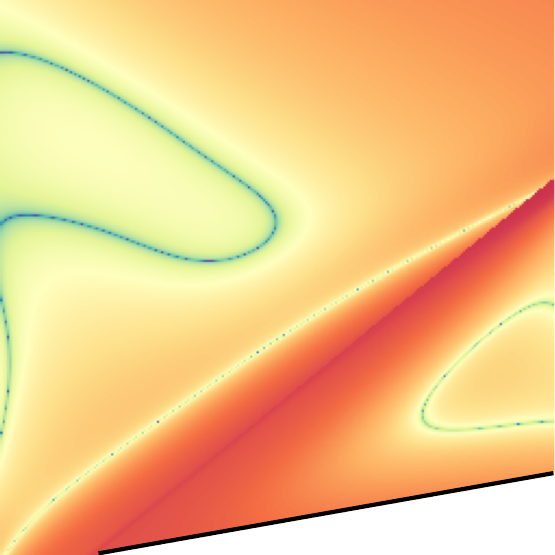};

        \nextgroupplot[
            tick align=outside,
            tick pos=left,
            ymin=1e-3,
            ymax=1e3,
            legend style={at={(1.0,1.0)},anchor=north east,font=\footnotesize,},
            log basis x={10},
            log basis y={10},
            ymode=log,
            xtick style={color=black},
            xlabel=step,
            % ylabel=$\mathcal{L}$,
            % title=(c)
            ]
        \addplot [line width=1.0pt, TUMblue] table[x index = {10}, y index = {0}]
        {figures/appendix/forward_problem/pinn/loss_history_60000.txt};
        \addlegendentry{$E$}
        \addplot [line width=1.0pt, TUMorange] table[x index = {10}, y index = {6}]
        {figures/appendix/forward_problem/pinn/loss_history_60000.txt};
        \addlegendentry{$W$}
        \addplot [line width=1.0pt, TUMgreen] table[x index = {10}, y index = {9}]
        {figures/appendix/forward_problem/pinn/loss_history_60000.txt};
        \addlegendentry{$\mathbf{u}\cdot \mathbf{n}$}
        \addplot [line width=1.0pt, black, dashed] coordinates {(20000,1e-3) (20000,1e3)};
    \end{groupplot}
    % \node[above, yshift=1cm] at ($(group c1r1.north east)!0.5!(group c2r1.north west)$) {Compression ramp};
    % \node[above, yshift=1cm] at ($(group c3r1.north east)!0.5!(group c4r1.north west)$) {Expansion ramp};
\end{tikzpicture}
