# Supplementary material for: Data-driven shape inference in three-dimensional steady state supersonic flows using ODIL and JAX-Fluids
Source: arXiv:2408.10094 source file (2025-06-18)
Supplement: Supplementary file 3 [file loss_history.tex]

\begin{tikzpicture}

    \begin{groupplot}[
        group style={group size=2 by 1, horizontal sep=1.5cm},
        width=5.0cm, height=5.0cm]
      
    \nextgroupplot[
    tick align=outside,
    tick pos=left,
    legend style={at={(0.99,0.99)},draw=none,anchor=north east,font=\tiny},
    xtick style={color=black},
    ymin=1e-12, ymax=1e4,
    % xmin=0.0, xmax=1e5,
    log basis x={10},
    log basis y={10},
    xtick={0,40000,30000},
    % xmode=log,
    ymode=log,
    xlabel=step,
    ylabel=$\omega \mathcal{L}$,
    title=(a)
    ]

    \addplot [line width=0.5pt, blue] table[skip first n=1,
        x index = {0}, y index = {2}
        ] {figures/flow_field_reconstruction/expansionramp/loss_history_30000.txt};
    \addlegendentry{$E$};
    \addplot [line width=0.5pt, red] table[skip first n=1,
        x index = {0}, y index = {3}
        ] {figures/flow_field_reconstruction/expansionramp/loss_history_30000.txt};
    \addlegendentry{$W$};
    \addplot [line width=0.5pt, lime] table[skip first n=1,
        x index = {0}, y index = {4}
        ] {figures/flow_field_reconstruction/expansionramp/loss_history_30000.txt};
    \addlegendentry{$S$};
    \addplot [line width=0.5pt, magenta] table[skip first n=1,
        x index = {0}, y index = {6}
        ] {figures/flow_field_reconstruction/expansionramp/loss_history_30000.txt};
    \addlegendentry{$T_0$};
    \addplot [line width=0.5pt, black, dashed] coordinates {(10000,1e-12) (10000,1e4)};
    % \addplot [line width=0.5pt, black, dotted] coordinates {(20000,1e-12) (20000,1e4)};

    \nextgroupplot[
        tick align=outside,
        tick pos=left,
        xtick style={color=black},
        ymin=1e-10, ymax=1e4,
        % xmin=0.0, xmax=1e5,
        log basis x={10},
        log basis y={10},
        xtick={0,40000,30000},
        % xmode=log,
        ymode=log,
        xlabel=step,
        title=(b)
        % ylabel=$\mathcal{L}$
        ]
    
    \addplot [line width=0.5pt, blue] table[skip first n=1,
    x index = {0}, y index = {2}
    ] {figures/flow_field_reconstruction/compressionramp/loss_history_30000.txt};
    \addplot [line width=0.5pt, red] table[skip first n=1,
        x index = {0}, y index = {3}
        ] {figures/flow_field_reconstruction/compressionramp/loss_history_30000.txt};
    \addplot [line width=0.5pt, lime] table[skip first n=1,
        x index = {0}, y index = {4}
        ] {figures/flow_field_reconstruction/compressionramp/loss_history_30000.txt};
    \addplot [line width=0.5pt, magenta] table[skip first n=1,
        x index = {0}, y index = {6}
        ] {figures/flow_field_reconstruction/compressionramp/loss_history_30000.txt};
    \addplot [line width=0.5pt, black, dashed] coordinates {(10000,1e-12) (10000,1e4)};
    % \addplot [line width=0.5pt, black, dotted] coordinates {(20000,1e-12) (20000,1e4)};

    \end{groupplot}
\end{tikzpicture}
