# Supplementary material for: Data-driven shape inference in three-dimensional steady state supersonic flows using ODIL and JAX-Fluids
Source: arXiv:2408.10094 source file (2025-06-18)
Supplement: Supplementary file 4 [file interface_reconstruction.tex]

\begin{tikzpicture}
    \draw[thick, black] (0,0) -- (0,2) node[at end, circle, draw=TUMblue] {} -- (2,2) node[at end, circle, draw=TUMblue] {} -- (2,0) node[at end, circle, draw=TUMblue] {} -- (0,0) node[at end, circle, draw=TUMblue, fill=TUMblue] {};
    \draw[thick, dashed] (1.0,0.0) -- (0.0,1.0);
    \draw[thick, black] (3,0) -- (3,2) node[at end, circle, draw=TUMblue, fill=TUMblue] {} -- (5,2) node[at end, circle, draw=TUMblue] {} -- (5,0) node[at end, circle, draw=TUMblue] {} -- (3,0) node[at end, circle, draw=TUMblue, fill=TUMblue] {};
    \draw[thick, dashed] (3.8,0.0) -- (4.2,2.0);
    \draw[thick, black] (6,0) -- (6,2) node[at end, circle, draw=TUMblue, fill=TUMblue] {} -- (8,2) node[at end, circle, draw=TUMblue] {} -- (8,0) node[at end, circle, draw=TUMblue, fill=TUMblue] {} -- (6,0) node[at end, circle, draw=TUMblue] {};
    \draw[thick, dashed] (6.0,0.5) -- (7.0,2.0);
    \draw[thick, dashed] (7.2,0.0) -- (8.0,0.8);
\end{tikzpicture}
